# Supplementary material for: Prompt-delayed $\gamma$-ray spectroscopy of neutron-rich $^{119,121}$In isotopes
Source: arXiv:2007.10043 ancillary file (2020-07-20)
Supplement: Supplementary file 1 [file PaperInSupp.pdf]

# Prompt-delayed $\gamma$ -ray spectroscopy of neutron-rich $^{119,121}\text{In}$ isotopes Supplemental Material

S. Biswas,<sup>1</sup> A. Lemasson,<sup>1,\*</sup> M. Rejmund,<sup>1</sup> A. Navin,<sup>1</sup> Y.H. Kim,<sup>1,†</sup> C. Michelagnoli,<sup>1,†</sup> I. Stefan,<sup>2</sup>  
R. Banik,<sup>3,4</sup> P. Bednarczyk,<sup>5</sup> Soumik Bhattacharya,<sup>3,4</sup> S. Bhattacharyya,<sup>3,4</sup> E. Clément,<sup>1</sup> H.  
L. Crawford,<sup>6</sup> G. de France,<sup>1</sup> P. Fallon,<sup>6</sup> G. Frémont,<sup>1</sup> J. Goupil,<sup>1</sup> B. Jacquot,<sup>1</sup> H.J. Li,<sup>1</sup>  
J. Ljungvall,<sup>2</sup> A. Maj,<sup>5</sup> L. Ménager,<sup>1</sup> V. Morel,<sup>1</sup> R. Palit,<sup>7</sup> R.M. Pérez-Vidal,<sup>8</sup> and J. Ropert<sup>1</sup>  
<sup>1</sup>GANIL, CEA/DRF-CNRS/IN2P3, Bd Henri Becquerel, BP 55027, F-14076 Caen Cedex 05, France  
<sup>2</sup>Université Paris-Saclay, CNRS/IN2P3, IJCLab, 91405 Orsay, France  
<sup>3</sup>Variable Energy Cyclotron Centre, 1/AF Bidhan Nagar, Kolkata 700064, India  
<sup>4</sup>Homi Bhabha National Institute, Training School Complex, Anushaktinagar, Mumbai-400094, India  
<sup>5</sup>Institute of Nuclear Physics PAN, 31-342 Kraków, Poland  
<sup>6</sup>Nuclear Science Division, Lawrence Berkeley National Laboratory, Berkeley, California 94720, USA  
<sup>7</sup>Department of Nuclear and Atomic Physics, Tata Institute of Fundamental Research, Mumbai, 400005, India  
<sup>8</sup>Instituto de Física Corpuscular, CSIC-Universitat de València, E-46980 València, Spain  
( Dated: July 6, 2020)

Supplemental material including tabulated values of energies of the levels and  $\gamma$ -ray transitions energies and intensities reported in this work.

The energies and intensities of the  $\gamma$ -ray transitions observed in the present work for  $^{119}\text{In}$  and  $^{121}\text{In}$  are given respectively in the Tables I and II. The energy uncertainty of prompt and delayed  $\gamma$  rays is  $\sim 1$  keV [1, 2]. The efficiencies for the prompt and delayed  $\gamma$  rays were determined separately. The spin-parities were assigned based on systematics and shell model calculations. The detailed information on the extraction of intensities is given below.

## $^{119}\text{In}$

Prompt  $\gamma$ -rays : the intensity of the strongest low lying 1204 keV transition was normalized to 100. The intensities of the other  $\gamma$ -ray transitions (721, 422, 636 and 740) were normalized relative to 1204 keV transition. As 207 and 336 keV transitions lie just above the isomers ( $19/2^-$ ) and ( $25/2^+$ ), respectively, these have been normalized to 100. The intensities of the 289, 145, 599, 499, 1098, 313 and 511 keV transitions were normalized relative to the 207 keV transition. Whereas the intensity of the 460 keV transition was normalized relative to the 336 keV transition. The 60 and 64 keV transitions were not observed in the present data and so their intensities could not be determined.

Delayed  $\gamma$ -rays : the intensity of the 1204 keV transition was normalized to 100. The intensities of 1025, 178, 1020, 928, 94, 218 and 152 keV transitions were normalized relative to the 1204 keV transition.

## $^{121}\text{In}$

Prompt  $\gamma$ -rays : the intensity of the strongest low lying 1181 keV transition was normalized to 100. The intensities of the other  $\gamma$ -ray transitions (988, 420, 640, 1052, 160 and 1021 keV) were normalized relative to the 1181 keV transition. The 169 and 326 keV transitions lie just above the isomers ( $19/2^-$ ) and ( $25/2^+$ ), respectively, they have been normalized to 100. The intensities of the 110, 573, 543, and 1116 keV transitions are normalized relative to the 169 keV transition. Whereas the 352 and 763 keV transitions were normalized based on the 326 keV transition. Two transitions of unknown energies X and Y (as Reported in Ref.[3]) could not be observed using the present experimental setup.

Delayed  $\gamma$ -rays : the intensity of the 1181 keV transition was normalized to 100. The intensities of the 953, 214 and 99 keV transitions were normalized relative to the 1181 keV transition. The 1021 and 160 keV transitions are not observed in the delayed spectrum very clearly and hence these two transitions were determined from the prompt  $\gamma$ -ray spectra. The 1052 keV transition was not observed in the delayed spectrum at all.

\* [lemasson@ganil.fr](mailto:lemasson@ganil.fr)

† Present address: Institut Laue-Langevin, F-38042 Grenoble Cedex, France

TABLE I. Properties of the transitions assigned to  $^{119}\text{In}$  obtained in this work. The relative intensities for the prompt ( $E_{\gamma_P}$ ) and delayed ( $E_{\gamma_D}$ ) transitions are reported, ordered by decreasing intensity.

| $E_{\gamma_P}$ | $I_\gamma$ | $J_i^\pi \rightarrow J_f^\pi$   | $E_i$ | $E_f$ |
|----------------|------------|---------------------------------|-------|-------|
| 207            | 100        | $(21/2^-) \rightarrow (19/2^-)$ | 2493  | 2286  |
| 289            | 81(2)      | $(23/2^-) \rightarrow (21/2^-)$ | 2782  | 2493  |
| 145            | 77(3)      | $(25/2^-) \rightarrow (23/2^-)$ | 2927  | 2782  |
| 599            | 38(2)      | $(27/2^-) \rightarrow (25/2^-)$ | 3526  | 2927  |
| 499            | 15(3)      | $(29/2^-) \rightarrow (27/2^-)$ | 4025  | 2927  |
| 1098           | 27(3)      | $(29/2^-) \rightarrow (25/2^-)$ | 4025  | 2927  |
| 313            | 10(4)      |                                 |       |       |
| 511            | 9(4)       |                                 |       |       |
| 1204           | 100        | $(13/2^+) \rightarrow 9/2^+$    | 1204  | 0     |
| 721            | 57(3)      | $(7/2^+) \rightarrow 9/2^+$     | 721   | 0     |
| 422            | 45(3)      | $(11/2^+) \rightarrow (7/2^+)$  | 1143  | 721   |
| 636            | 34(4)      | $(15/2^+) \rightarrow (11/2^+)$ | 1779  | 1143  |
| 740            | 11(4)      | $(19/2^+) \rightarrow (15/2^+)$ | 2519  | 1779  |
| 336            | 100        | $(27/2^+) \rightarrow (25/2^+)$ | 2992  | 2656  |
| 460            | 68(2)      | $(29/2^+) \rightarrow (27/2^+)$ | 3452  | 2992  |
| <hr/>          |            |                                 |       |       |
| $E_{\gamma_D}$ | $I_\gamma$ | $J_i^\pi \rightarrow J_f^\pi$   | $E_i$ | $E_f$ |
| 1204           | 100        | $(13/2^+) \rightarrow 9/2^+$    | 1204  | 0     |
| 1020           | 55(20)     | $(17/2^+) \rightarrow (13/2^-)$ | 2224  | 1204  |
| 928            | 44(21)     | $(15/2^-) \rightarrow (13/2^+)$ | 2132  | 1204  |
| 94             | 40(22)     | $(17/2^-) \rightarrow (15/2^-)$ | 2226  | 2132  |
| 218            | 37(23)     | $(21/2^+) \rightarrow (19/2^-)$ | 2504  | 2286  |
| 152            | 33(24)     | $(25/2^+) \rightarrow (21/2^+)$ | 2656  | 2504  |
| 1025           | 15(7)      | $(11/2^+) \rightarrow 9/2^+$    | 1025  | 0     |
| 178            | 8(5)       | $(13/2^+) \rightarrow (11/2^+)$ | 1204  | 1025  |

TABLE II. Properties of the  $\gamma$ -ray transitions assigned to  $^{121}\text{In}$  obtained in this work. The relative intensities for the prompt ( $E_{\gamma_P}$ ) and delayed ( $E_{\gamma_D}$ ) transitions are reported, ordered by decreasing intensity. The X and Y energies refers respectively to the energy of the unobserved  $(17/2^-) \rightarrow (15/2^-)$  and  $(19/2^-) \rightarrow (17/2^-)$  transitions as reported in Ref. [3]. Because of these unobserved transitions, excitation energies of levels above the  $15/2^-$  level are not determined.

| $E_{\gamma_P}$ | $I_\gamma$ | $J_i^\pi \rightarrow J_f^\pi$   | $E_i$          | $E_f$          |
|----------------|------------|---------------------------------|----------------|----------------|
| 1181           | 100        | $(13/2^+) \rightarrow 9/2^-$    | 1181           | 0              |
| 988            | 35(2)      | $(7/2^+) \rightarrow 9/2^+$     | 988            | 0              |
| 1021           | 37(2)      | $(11/2^+) \rightarrow 9/2^+$    | 1021           | 0              |
| 1052           | 25(3)      | $(17/2^+) \rightarrow (13/2^+)$ | 2233           | 1181           |
| 420            | 16(2)      | $(11/2^-) \rightarrow (7/2^+)$  | 1408           | 988            |
| 160            | 11(5)      | $(13/2^+) \rightarrow (11/2^+)$ | 1181           | 1021           |
| 640            | 10(2)      | $(15/2^+) \rightarrow (11/2^+)$ | 2048           | 1408           |
| 169            | 100        | $(21/2^-) \rightarrow (19/2^-)$ | $2303 + X + Y$ | $2134 + X + Y$ |
| 361            | 85(3)      | $(23/2^-) \rightarrow (21/2^-)$ | $2664 + X + Y$ | $2303 + X + Y$ |
| 110            | 57(4)      | $(25/2^-) \rightarrow (23/2^-)$ | $2774 + X + Y$ | $2664 + X + Y$ |
| 573            | 35(4)      | $(27/2^-) \rightarrow (25/2^-)$ | $3347 + X + Y$ | $2774 + X + Y$ |
| 543            | 20(4)      | $(29/2^-) \rightarrow (27/2^-)$ | $3890 + X + Y$ | $3347 + X + Y$ |
| 1116           | 18(5)      | $(29/2^-) \rightarrow (25/2^-)$ | $3890 + X + Y$ | $2774 + X + Y$ |
| 326            | 100        | $(27/2^+) \rightarrow (25/2^+)$ | $2773 + X + Y$ | $2447 + X + Y$ |
| 352            | 69(3)      | $(29/2^+) \rightarrow (27/2^+)$ | $3125 + X + Y$ | $2773 + X + Y$ |
| 763            | 28(3)      | $(31/2^+) \rightarrow (29/2^+)$ | $3888 + X + Y$ | $3125 + X + Y$ |
| <hr/>          |            |                                 |                |                |
| $E_{\gamma_D}$ | $I_\gamma$ | $J_i^\pi \rightarrow J_f^\pi$   | $E_i$          | $E_f$          |
| 1181           | 100        | $(13/2^+) \rightarrow 9/2^-$    | 1181           | 0              |
| 953            | 40(18)     | $(15/2^-) \rightarrow (13/2^+)$ | 2134           | 1181           |
| 214            | 25(13)     | $(21/2^+) \rightarrow (19/2^-)$ | $2348 + X + Y$ | $2134 + X + Y$ |
| 99             | 10(5)      | $(25/2^+) \rightarrow (21/2^+)$ | $2447 + X + Y$ | $2348 + X + Y$ |

- 
- [1] Y. H. Kim, A. Lemasson, M. Rejmund, A. Navin, S. Biswas, C. Michelagnoli, I. Stefan, R. Banik, P. Bednarczyk, S. Bhattacharya, S. Bhattacharyya, E. Clément, *et al.*, [Eur. Phys. J. A \*\*53\*\*, 162 \(2017\)](#)
- [2] S. Biswas, A. Lemasson, M. Rejmund, A. Navin, Y. H. Kim, C. Michelagnoli, I. Stefan, R. Banik, P. Bednarczyk, S. Bhattacharya, S. Bhattacharyya, E. Clément, *et al.*, [Phys. Rev. C \*\*99\*\*, 064302 \(2019\)](#)
- [3] R. Lucas, M.-G. Porquet, T. Venkova, I. Deloncle, M. Houry, C. Theisen, A. Astier, A. Bauchet, S. Lalkovski, G. Barreau, N. Buorn, T. Doan, *et al.*, [Eur. Phys. J. A \*\*15\*\*, 315 \(2002\)](#)
